# Supplementary material for: PerSim: Data-Efficient Offline Reinforcement Learning with Heterogeneous Agents via Personalized Simulators
Source: arXiv:2102.06961 source file (2021-11-10)
Supplement: Supplementary file 1 [file appendix_proofs.tex]

\section{Theoretical Results}\label{appendix:sec:proof}

\subsection{Proof of Theorem \ref{thm:representation}} 
\begin{proof}
%Consider any coordinate $d$. 
 We will construct a low-rank order-four tensor $\Tc \in \Rb^{N \times |\Sc| \times |\Ac| \times D}$ by partitioning the latent parameter spaces associated with agents, states, actions, and the {\color{red} $d$-th} coordinate of the expected next state. 
 As we will see, it would be helpful to think of $\Tc$ as a composition of $D$ order-three tensors, denoted as $\Tc^{(d)} \in \Rb^{N \times |\Sc| \times |\Ac|}$, corresponding to each coordinate $d$.   
 In doing so, we will demonstrate that each frontal slice of $\Tc^{(d)}$ is a low-rank matrix and only a subset of the $| \Ac|$ frontal slices of $\Tc^{(d)}$ are distinct. 
 Similarly, we will prove that a subset of the $D$ order-three tensors $\Tc^{(d)}$ will be distinct as well. 
 Together, these observations establish the low-rank property of $\Tc$. 
 Finally, we will complete the proof by showing that $\Xc$ is entry-wise arbitrarily close to $\Tc$.

{\bf Partitioning the latent spaces to construct $\Tc$.} 
Fix some $\delta_1, \delta_3, \delta_4 > 0$. 
Since the latent row parameters $\theta_n$ come from a compact space $[0,1]^{d_1}$, we can construct a finite covering or partitioning $P_1(\delta_1) \subset [0,1]^{d_1}$ such that for any $\theta_n \in [0,1]^{d_1}$, there exists a $\theta_{n'} \in P_1(\delta_1)$ satisfying $\|\theta_n - \theta_{n'} \|_2 \le \delta_1$. 
By the same argument, we can construct a partitioning $P_3(\delta_3) \subset [0,1]^{d_3}$ such that $\| \omega_a - \omega_{a'} \|_2 \le \delta_3$ for any $\omega_a \in [0,1]^{d_3}$ and some $\omega_{a'} \in P_3(\delta_3)$; 
similarly, $P_4(\delta_4) \subset [0,1]^{d_4}$ such that $\| \alpha_d - \alpha_{d'} \|_2 \le \delta_4$ for any $\alpha_d \in [0,1]^{d_4}$ and some $\alpha_{d'} \in P_4(\delta_4)$. 

For each $\theta_n$, let $p_1(\theta_n)$ denote the unique element in $P_1(\delta_1)$ that is closest to $\theta_n$. 
At the same time, we define $p_3(\omega_a)$ and $p_4(\alpha_d)$ as the corresponding elements in $P_3(\delta_3)$ and $P_4(\delta_4)$ that are closest to $\omega_a$ and $\alpha_d$, respectively. 
We now construct our tensor $\Tc = [T_{nsad}]$ by defining its $(n,s,a,d)$-th entry as 
$T_{nsad} =  f(p_1(\theta_n), \rho_s, p_3(\omega_a), p_4(\alpha_d))$.

{\bf Establishing the low-rank property of $\Tc$.} 
Let us fix a coordinate $d$ to consider $\Tc^{(d)} = [T_{nsad}]_{n \in [N], s \in [\Sc], a \in [\Ac]} \in \Rb^{N \times |\Sc| \times |\Ac|}$, and fix a frontal slice $a$ of $\Tc^{(d)}$. 
Now, consider any two rows of $\Tc^{(d)}_{\cdot, \cdot, a}$, say $n$ and $n'$. 
If $p_1(\theta_n) = p_1(\theta_{n'})$, then rows $n$ and $n'$ of $\Tc^{(d)}_{\cdot, \cdot, a}$ are identical. 
Hence, there at most $|P_1(\delta_1)|$ distinct rows in $\Tc^{(d)}_{\cdot, \cdot, a}$, and thus  $\text{rank}(\Tc^{(d)}_{\cdot, \cdot, a}) \le |P_1(\delta_1)|$. 
In words, each frontal slice of $\Tc^{(d)}$ is a low-rank matrix with its rank bounded above by $|P_1(\delta_1)|$. 

Next, consider any two frontal slices $a$ and $a'$ of $\Tc^{(d)}$. If $p_3(\omega_a) = p_3(\omega_{a'})$, then for all $(n,s)$, we have 
$
	T_{nsad} = f(p_1(\theta_n), \rho_s, p_3(\omega_a), p_4(\alpha_d)) = f(p_1(\theta_n), \rho_s, p_3(\omega_{a'}),  p_4(\alpha_d)) = T_{nsa'd}.
$
In words, the $a$-th frontal slice of $\Tc^{(d)}$ is equivalent to the $a'$-th frontal slice of $\Tc^{(d)}$.
Hence, $\Tc^{(d)}$ has at most $|P_3(\delta_3)|$ distinct frontal slices.

Following the arguments above, consider any two coordinates $d$ and $d'$. 
If $p_4(\alpha_d) = p_4(\alpha_{d'})$, then 
$
	T_{nsad} = f(p_1(\theta_n), \rho_s, p_3(\omega_a), p_4(\alpha_d)) = f(p_1(\theta_n), \rho_s, p_3(\omega_{a}), , p_4(\alpha_{d'})) = T_{nsad'}.
$
This establishes that $\Tc$ can be decomposed into at most $|P_4(\delta_4)|$ distinct order-three tensors. 

To recap, we have established that all of the frontal slices $\Tc^{(d)}_{\cdot, \cdot, a}$ of $\Tc^{(d)}$ are low-rank matrices, and only a subset of the frontal slices of $\Tc^{(d)}$ are distinct. 
We have also proven that only a subset of the order-three tensors $\Tc^{(d)}$ are distinct. 
Therefore, it follows that the canonical polyadic (CP) rank of $\Tc$ is bounded by the product of the maximum matrix rank of any slice of $\Tc^{(d)}$ with the number of distinct slices in $\Tc^{(d)}$ and the number of distinct order-three tensors in $\Tc$. 
More specifically, 
$
	\text{rank}(\Tc) \le |P_1(\delta_1)| \cdot |P_3(\delta_3)| \cdot |P_4(\delta_4)|. 
$

%{\color{orange} include short proof on rank inequality} 
%where $C$ is a constant that depends on the latent spaces $[0,1]^{d_1}$ and $[0,1]^{d_3}$, the dimensions $d_1$ and $d_3$, and the Lipschitz constant $\mathcal{L}$. We highlight that the bound on the tensor rank does not depend on the dimensions of $\tT$. 

{\bf $\Xc$ is well approximated by $\Tc$.}
Here, we bound the maximum difference of any entry in $\Xc$ from $\Tc$. 
Using the Lipschitz property of $f$ (Assumption \ref{assumption:f_properties}), we obtain for any $(n,s,a,d)$, 
\begin{align}
	|X_{nsad} - T_{nsad}| &= | f(\theta_n, \rho_s, \omega_a, \alpha_d) - f(p_1(\theta_n), \rho_s, p_3(\omega_a), p_4(\alpha_d))|
	\\ &\le L \cdot \left( \| \theta_n - p_1(\theta_n) \|_2 + \| \omega_a - p_3(\omega_a) \|_2 + \| \alpha_d - p_4(\alpha_d) \|_2 \right) 
	\\ &\le L \cdot (\delta_1 + \delta_3 + \delta_4). 
\end{align}
This proves $\Xc$ is entry-wise arbitrarily close to $\Tc$.

{\bf Concluding the proof.} 
By the Lipschitz property of $f$ and the compactness of the latent spaces, it follows that $|P_1(\delta_1)| \le C  \delta_1^{-d_1}, |P_3(\delta_3)| \le C  \delta_3^{-d_3}, |P_1(\delta_4)| \le C  \delta_4^{-d_4}$, where $C$ is an absolute constant. 
% constant that depends only on the space $[0,1]^{d_1}$, ambient dimension $d_1$, and Lipschitz constant $L$. 
%
% Similarly, $|P_3(\delta_3)| \le C_3  \delta_3^{-d_3}$, where $C_3$ is an absolute constant.
% % that depends only on $[0,1]^{d_3}$, $d_3$, and $L$; 
% Lastly $|P_4(\delta_4)| \le C_4  \delta_4^{-d_4}$, where $C_4$ is a constant that depends only on $[0,1]^{d_4}$, $d_4$, and $L$. 
%
As such, we can bound the tensor rank $r = \text{rank}(\Tc)$ as $r \le C \delta_1^{-d_1} \delta_3^{-d_3} \delta_4^{-d_4}$. Importantly, $r$ does not depend on the dimensions of $\Tc$.
Further, by definition of CP-rank, this allows us to write any entry of $\Tc$ as 
\begin{align}
    T_{nsad} &= \sum_{\ell=1}^r u_{n\ell} v_{s\ell} w_{a \ell} q_{d \ell}
    = \sum_{\ell=1}^r u_{n\ell} v^{(d)}_{s\ell} w_{a \ell},
\end{align}
where $v^{(d)}_{s \ell} = v_{s\ell} q_{d\ell}$. 
Consequently, for any coordinate $d$, we can write 
\begin{align}
    \Tc^{(d)} = \sum_{\ell=1}^r u_{\ell} \otimes v^{(d)}_\ell \otimes w_\ell, 
\end{align} 
where $u_\ell \in \Rb^{N}$, $v^{(d)}_\ell \in \Rb^{|\Sc|}$, and $w_\ell \in \Rb^{|\Ac|}$. 
Observing that 
$\| \Xc^{(d)} - \Tc^{(d)}\|_{\max} \le \| \Xc - \Tc \|_{\max}$ and 
$\text{rank}(\Tc^{(d)}) \le \text{rank}(\Tc)$, and setting $\delta = \delta_1 = \delta_3 = \delta_4$ completes the proof. 

%Setting $\delta = \delta_1 = \delta_3 = \delta_4$ and observing that the partitioning of the latent agent and action spaces is invariant to $d$ completes the proof. 
\end{proof}

\subsection{Proof of Proposition  \ref{proposition:example}} 

\begin{proof}
To show that $\text{rank}(\Xc^{(d)}) = 3$ for $d \in \{1,2\}$, it suffices to find $u_{n \cdot} , v_{s \cdot}^{(1)}, v_{s \cdot}^{(2)} , w_{a \cdot} \in \Rb^3$ such that $X_{nsad} = \sum_{\ell=1}^r u_{n\ell} v^{(d)}_{s\ell} w_{a \ell}$ for any $n \in [N]$, $s = [s_{1},s_{2}] \in \Sc$,  and $a \in \Ac$. 
Further, we require that $u_{n \cdot}$ can only depend on agent $n$, i.e., not on the action or state. 
Analogously, 
%$v_{s \cdot}^{(1)}, v_{s \cdot}^{(2)} , w_{a \cdot}$ have analogous requirements on them -- 
%
$v_{s \cdot}^{(1)}, v_{s \cdot}^{(2)}$ can only depend on the state, and $w_{a \cdot}$ can only depend the action. 
Towards this, consider the following factors: 
\begin{align*}
u_{n \cdot} = \begin{bmatrix}
 {1} & {g_n} & {1}
\end{bmatrix}, \qquad  
w_{a \cdot} = \begin{bmatrix}
{1} & {1} & {a}
\end{bmatrix}, \qquad 
v_{s \cdot}^{(1)} =  \begin{bmatrix}
{s_{1} + s_{2}} &   {-\frac{\cos(3s_{1})}{2}}  & {\frac{1}{2}}  \\
\end{bmatrix},  \qquad 
v_{s \cdot}^{(2)} =  \begin{bmatrix}
{ s_{2}}  & {-\cos(3s_{1})} & {1}
\end{bmatrix}. 
\end{align*}
Recalling that $ X_{nsa1} = {  s_{1} +
\  s_{2} } { -\frac{g_n\cos(3s_{1})}{2}} { +\frac{a}{2} } $ and $X_{nsa2} = { s_{2}}   {- g_n\cos(3s_{1})} + { a}$ completes the proof.  
\end{proof}
